# Supplementary material for: Exploring Data-Driven Advocacy in Home Health Care Work
Source: arXiv:2501.16305 source file (2025-01-27)
Supplement: Supplementary file 1 [file 7-appendix.tex]

\newpage
\appendix

\section{Sample Visualizations}

% \subsection{Ideation Sessions}
% \begin{figure}[h!]
%     % \centering
%     \includegraphics[width=.75\linewidth]{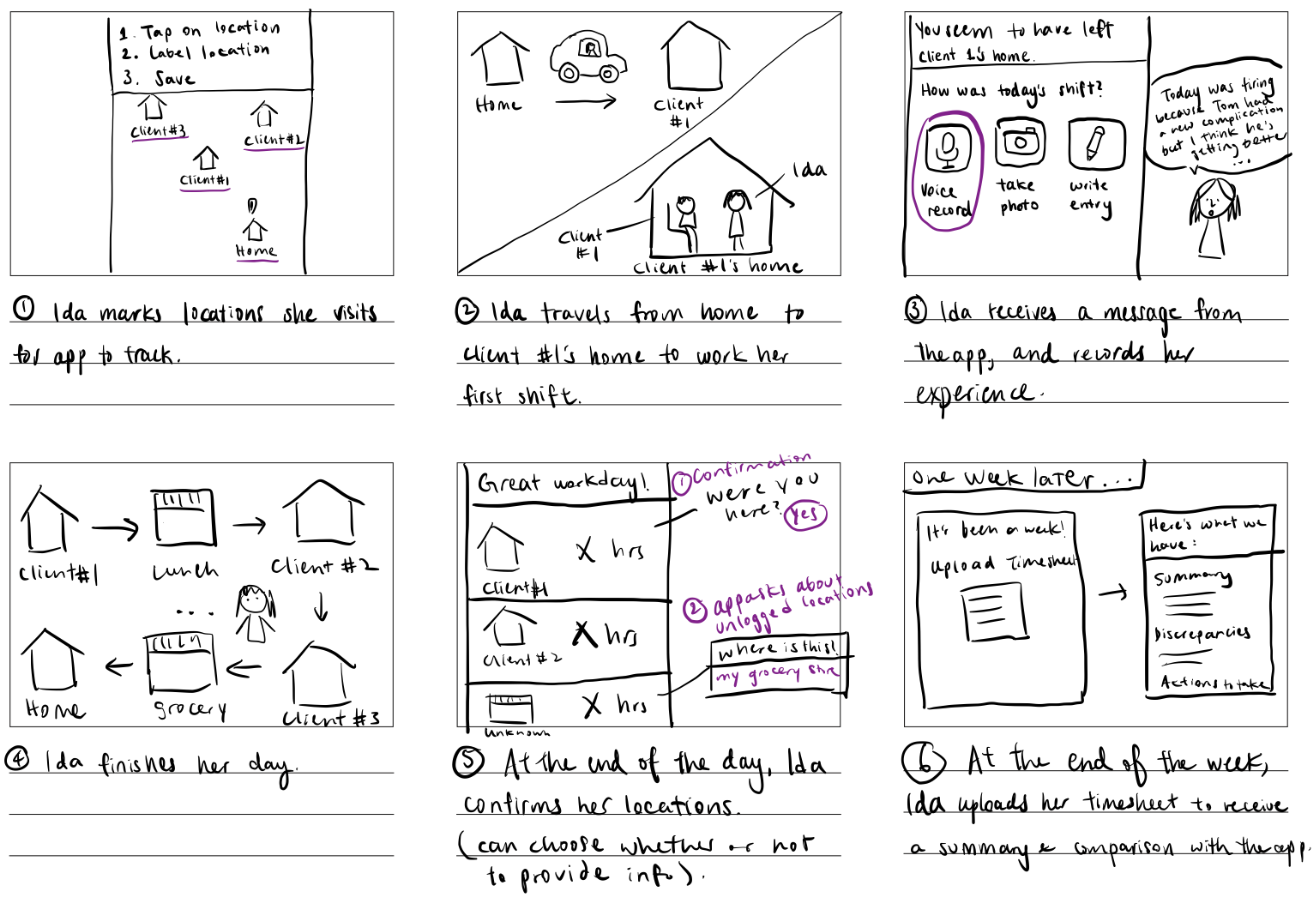}
%     \caption{Storyboard depicting the proposed data collection flow presented in the advocate focus groups.}
%     \Description[Six panels describing a home care worker Ida's use of a sample intervention.]{In the first panel, there is an image of an where Ida marks locations she visits like her home and clients' homes. In the second panel, there is an image showing Idea traveling from her home to client \#1's home to work her first shift. The third panel shows idea receiving a message from the app to record her experience at her shift. In the fourth panel, Ida travels between her clients homes, lunch, and the grocery before returning home to finish her day. in the fifth panel, the app shows idea confirming her locations for the day and choosing whether or not to provide the information. Finally, the sixth panel shows Ida uploading her timesheet and paystub one week later to receive a summary of her wages and hours by the app.}
%     \label{fig:storyboard} 
%     % \small 
%     % As part of the ideation sessions, the advocates were walked through a storyboard depicting what an ideal workflow could look like for data collection and asked to point out areas they might have concerns about.
% \end{figure}
% Overview

\subsection{Intervention Development}
\label{sec:development-figs}

% As part of the intervention development, we added a few features to the WeClock application in order to make it match the home care context. 

\begin{figure}[h!]
    \centering
    \includegraphics[width=0.85\linewidth]{img-journal.png}
    \caption{Sample questions from the daily work journal}
    \label{fig:journal}
    \Description[Four screenshots from the WeClock application with questions workers were asked to complete]{This figure shows four screenshots. The first screenshot has the question "How was your work day?" and in smaller text a description "How do you feel emotionally and physically? Did anything of note happen today?" There is then a textbox with part of a sample answer "...two clients and I had a great day with..." The second screenshot has the question "Did you spend any extra time today on work outside of your hours?" with the options "Arrived early or left late", "Contacted client", "Ran additional errands", "Contacted your agency", "Fixed issues with pay", "Did work training," "Other," and "None." The third screenshot has the question "Do any of these reasons explain why you did extra work today?" with the options "Worries about your job," "Maintaining good relations," "Challenging relationships," "Mistake in the care plan," "Issues with technology," "Difficulty reaching agency," "Other," and "None." The fourth and final screenshot has the question "Which of the following is true about your work today?" with options "I feel satisfied with my work," "I gave the level of care I wanted to," "I had control of my work," "I feel emotionally drained," "My work impacted my personal life," "Other," and "None."}
    \small
    One of the changes we made to WeClock was to change the questions in the daily journal to be more detailed and related to home care work. We present some of the examples of the questions the workers were asked.
\end{figure}

\begin{figure}[h!]
    \centering
    \includegraphics[width=0.85\linewidth]{img-data-upload.png}
    \caption{Workflows for uploading data, including manual and automatic upload options}
    \label{fig:upload}
    \Description[Five screenshots from the app on how to upload data manually or automatically]{This figure contains two sections: the "Manual" section, which shows how to upload data manually, and the "Automatic" section, which demonstrates how to upload data automatically. The manual option includes four screenshots on the left. The first screenshot shows different types of data collected, such as location (geo_logging) and app usage. Workers can click the up arrow icon to upload data, leading to the second screen where they can select the first day of the data to be uploaded. After clicking 'Next,' they are taken to the third screen to choose the last day. The final page allows them to choose which days of the week they work. The automatic option on the right shows the settings page, where users can check a box to enable automatic data uploads.}
    \small 
    These screenshots illustrate how workers can upload data either manually or automatically. Providing these options helped automate the data collection process, significantly reducing the burden on workers.
\end{figure}

\begin{figure}[h!]
    \centering
    \includegraphics[width=0.6\linewidth]{img-paystub.png}
    \caption{Workflow for uploading paystubs}
    \label{fig:paystub}
    \Description[Three screenshots from the app on how to upload paystubs]{The figure displays three screenshots from the app, showing the process for uploading timesheets/paystubs. The first screenshot features the date and a button to upload an image. The second screenshot navigates users to their gallery, where they can select the picture to upload. The final screenshot provides a text box where users can describe the image, whether it's a paystub, reimbursement, or the like.}
    \small 
By following these steps to upload their journal entries, workers were able to submit records of their schedules, which were later compared with GPS location data for quantitative analysis.
\end{figure}

\begin{figure}[h!]
    \centering
    \includegraphics[width=0.5\linewidth]{img-annotate.png}
    \caption{Workflow for annotating daily schedule}
    \label{fig:annotate}
    \Description[Two screenshots from the web tool used to annotate daily schedule]{The figure displays two screenshots. The first includes a map at the top with labels in certain locations that said "Place 1" through "Place 5." In the bottom half, there is a section for "Place 1" with a list of the dates and times the worker spent their time there. The worker is able to edit the name of the location, view the location, or remove the place. The second screenshot displaces a map at the top with one circle labeled with "Place 1." Below that, there is a list of dates ("8 Dec" "12 Dec" "13 Dec" "14 Dec") with "12 Dec" selected. Below that, there is and a list of times with some sections blocked with the name of a place (i.e., between 1am and 6am it says "Place 1 (4h)").}
    \small 
We tried out a tool with a few workers that would allow workers to annotate their daily schedules, including naming the locations they spent their time or removing it from the record. Additionally, workers were able to add notes about each of the locations.
\end{figure}

\subsection{Feedback Sessions}
\label{sec:feedback-figs}
